# Supplementary material for: AXI4MLIR: User-Driven Automatic Host Code Generation for Custom AXI-Based Accelerators
Source: arXiv:2312.14821 source file (2023-12-22)
Supplement: Supplementary file 1 [file 99-artifact-appendix.tex]

\appendix

\subsection{Artifact Evaluation}
This appendix describes how to reproduce our compilation flow, experiments, and results. We use a Git repository and Docker to install dependencies and build the \mlir compiler containing AXI4MLIR extensions from source. Additionally, we provide instructions on how to natively build AXI4MLIR in the project's~\href{https://github.com/AXI4MLIR/axi4mlir/blob/cgo2024_artifact/README.md}{README}.

\subsection{Checklist}
\begin{itemize}
    \item Benchmarks: Custom benchmarks, and ResNet18 and tinyBert models are included.
    \item Runtime environment: Tested on Ubuntu 22.04, though should be reproducible when run on any operating system as long as Docker is used.
    \item Hardware: Executing the experiments requires a PYNQ-Z1/Z2 board and FPGA bitmaps. Experiments were validated on both PYNQ-Z1 and Z2 boards running Pynq OS 4.19.0-xilinx-v2019. 
    \item Execution: Scripts to execute different experiments are provided.
    \item Metrics: Execution time, cache-references, branch instructions and other \lstinline{perf stat} metrics.
    \item Output: Experiments generate csv files, which are used to generate the graphs/plots.
    \item Experiments: See Appendix~\ref{ar-experiments}.
    \item How much disk space is required (approximately)?: Around 95GB after building all the required dependencies and AXI4MLIR.
    \item How much time is needed to prepare workflow (approximately)?: The compilation/installation phase takes around 30-60 mins when run on a 12-core 24-thread machine and 32GB DDR4 memory.
    \item How much time is needed to complete experiments (approximately)?: 20 mins.
    \item Publicly available?: Yes,~\url{https://github.com/AXI4MLIR/axi4mlir} and~\url{https://github.com/pnnl/soda-opt/pull/6}.
    \item Code licenses?: Apache License v2.0 with LLVM Exceptions and BSD2.
    \item Archived?: Yes,~\url{https://zenodo.org/doi/10.5281/zenodo.10204935}.

\end{itemize}

\subsection{Description}
\subsubsection{How to access?}
Clone repository from Github or download the zip file from Zenodo.

\subsubsection{Hardware dependencies}
Requires a PYNQ Z1/Z2 FPGA board to reproduce the results.

\subsubsection{Software dependencies}
All software dependencies are maintained via a Docker container.

\subsubsection{Datasets}
Data were generated depending on experiment and problem sizes.

\subsection{Installation}

This section requires you to have Unzip (option 1), Git (option 2), and Docker installed in your system.

\noindent \textbf{Option 1}: Download the file \lstinline{axi_mlir-*.zip} from~\href{https://zenodo.org/doi/10.5281/zenodo.10204935}{Zenodo}. Once downloaded, extract the contents and enter the project folder. 

\noindent \textbf{Option 2}: Alternatively, clone the correct version of the repository and update the submodules using the following Git commands.

\begin{lstlisting}[style=customMLIR,language=bash,numbers=none]
$ git clone -b cgo2024_artifact https://github.com/AXI4MLIR/axi4mlir.git
$ cd axi4mlir
$ git submodule init
$ git submodule update --depth=1
\end{lstlisting}

Once you have the repository setup, you can build the Docker image.

\begin{lstlisting}[style=customMLIR,language=bash,numbers=none]
$ ./build-docker.sh
\end{lstlisting}

After building the Docker image with needed dependencies installed, we are able to compile \mlir with AXI4MLIR extensions. Note this build process can take anywhere between 30 mins to an hour on a 12-core machine.

\begin{lstlisting}[style=customMLIR,language=bash,numbers=none]
$ ./compile-mlir.sh
\end{lstlisting}

Upon completion, you have AXI4MLIR compiled. The following subsections will help you reproduce the experiments reported in the paper using SystemC simulation to test functional correctness, and, if available, using a PYNQ Z1 board via remote access to collect performance metrics and re-generate the figures. Note that AXI4MLIR depends on system libraries for SystemC and cross-compilation, so target binaries must be built within Docker. Use the following command to enter the Docker container:

\begin{lstlisting}[style=customMLIR,language=bash,numbers=none]
$ ./start-docker.sh
\end{lstlisting}
  
\subsection{Experiments}
\label{ar-experiments}
\subsubsection{Ex1}

This experiment will reproduce code results for \textit{Figure~\ref{fig:exp-manual-vs-mlir-counters-optimized} \& Figure~\ref{fig:exp-manual-vs-mlir-genereated-all-best_mr_copy} 
}. This experiment uses the matmul accelerators v2 \& v3 with different accelerator sizes (8,16) across different matmul problems (M=N=K=[64, 128, 256]) and different dataflow strategies (Ns, As, Bs, Cs) with both AXI4MLIR generated code and handwritten C++ driver code.

\subsubsection{Ex2}
This experiment will reproduce code results for \textit{Figure~\ref{fig:v4_graph}}. This experiment uses the matmul accelerator v4 with different problem sizes, evaluating different tiling and dataflow strategies.

\subsubsection{Ex3}
This experiment will reproduce code results for \textit{Figure~\ref{fig:conv_graph}}. This experiment uses the convolution accelerator for all the convolution layers of ResNet18 with both AXI4MLIR generated code and handwritten C++ driver code. 

\subsubsection{Ex4}
This experiment will reproduce code results for \textit{Figure~\ref{fig:tinybert}}. This experiment uses the matmul accelerator v4 for all the matrix-multiplication layers of tinyBert, leveraging the AXI4MLIR generated code. In this experiment we observe end-to-end speedup over CPU execution of the model of a ''Nothing stationary`` strategy and the ''Best`` strategy during accelerator execution.

\subsection{SystemC Execution}

For demonstration and validation purposes, we have integrated a SystemC simulation infrastructure for our accelerators and enabled AXI4MLIR to generate code to drive these SystemC models.

In the folder for each experiment, we provide a script to generate driver code that will communicate with our SystemC models. We also provide a script to execute the experiments and verify correctness against CPU executions.

The following example is for \textit{Ex1}, but the same can be replicated for all the experiments.
Compile \& run SystemC-based experiment:
\begin{lstlisting}[style=customMLIR,language=bash,numbers=none]
$ ./start_docker
$ cd experiments/ex1/
$ ./compile_sysc.sh
$ ./run_sysc.sh
\end{lstlisting}

While running the SystemC-based experiment, you will see which task is being executed, and whether or not it passes the evaluation (generates correct results).

Additionally, during compilation, the script generates an intermediate representation for each task. This representation is saved within \path{./ex1_sysc/intermediate_[acc_name].mlir}.

\subsection{PYNQ Execution}
To run the experiments on the FPGA-SoC hardware, the user will require access to a PYNQ Z1/Z2 board. The instructions below can be followed by any future user by updating the ip-address, username, and ssh port for their PYNQ board within the \lstinline{pynq_send.sh} and \lstinline{pynq_run.sh} scripts. The experiments expect specific FPGA bitstreams implementing our accelerators. A user can download the bitstreams by executing the following commands \textit{inside the PYNQ board}.

\begin{lstlisting}[style=customMLIR,language=bash,numbers=none]
$ mkdir -p /home/axi4mlir/tester1
$ cd /home/axi4mlir/tester1
$ wget https://zenodo.org/records/10277700/ ...
  ... files/accelerator.bitmaps.zip?download=1 -O bits.zip
$ unzip bits.zip
\end{lstlisting}

During the artifact evaluation process using an FPGA-SoC, we provide remote access for the evaluator to a suitable device. In each experiment's folder, we provide scripts to cross-compile the experiments, copy, execute the compiled experiments on the device, and send experimental results back to the host machine.

The following example uses \textit{Ex1}, but the same process can be replicated for all the experiments.
To cross-compile and send relevant binaries to the PYNQ board, use the following commands (note: these scripts will require the evaluator to enter password for accessing the board multiple times):
\begin{lstlisting}[style=customMLIR,language=bash,numbers=none]
$ ./start_docker.sh
$ cd experiments/ex1/
$ ./compile_pynq.sh
$ ./pynq_send.sh
\end{lstlisting}

Execute experiments on the PYNQ board:
\begin{lstlisting}[style=customMLIR,language=bash,numbers=none]
$ ./pynq_run.sh
\end{lstlisting}

This script will provide remote access into the board using \lstinline{ssh}, load the correct bitstreams, and run all the tasks for the selected experiment.
After running the tasks, the script will copy the results back to the host device at \path{./ex1_pynq/results/.}
We can use these results (csv files) to regenerate graphs presented in the paper.

\subsection{Analysis}
Each experiment contains an ``analysis'' folder, which will contain the original data that was generated for the paper. Additionally, we include two Jupyter notebooks and two python scripts; both will generate the relevant graphs/plots presented in experiment. 

All dependencies are already installed inside the Docker container for the \textit{python scripts}. The python scripts can be executed with variations of the command below:

\begin{lstlisting}[style=customMLIR,language=bash,numbers=none]
$ ./start_docker.sh
$ cd experiments/ex1/analysis
$ python3 ex1-generate-paper-graphs.py
\end{lstlisting}

To use the notebooks, please set up the conda environment in your system using the following commands, or run the first cell (containing the pip3 command) of any of the notebooks to install the required Python packages.

\begin{lstlisting}[style=customMLIR,language=bash,numbers=none]
$ conda create -n bench python=3 pandas matplotlib numpy
$ conda activate bench
\end{lstlisting}

The notebook or script (marked with ``paper'') will use the original data and save figures in an output folder. The other notebook or script (marked with ``new'') will use generated results from the PYNQ board to recreate the figures.

\subsection*{Relevant Source Files}

Please check the~\href{https://github.com/AXI4MLIR/axi4mlir/blob/cgo2024_artifact/README.md}{README} for links to relevant files, implementing the following: Accel Dialect, New Attributes, Linalg to Accel transformation pass, Accel to AXI4MLIR DMA library transformation pass, tests, and an examples on how to setup the new mlir attributes, such as the \lstinline{opcode_map} and \lstinline{opcode_flow}, for accelerators with different capabilities.
